# Supplementary material for: Ten years of All-sky Neutrino Point-Source Searches
Source: arXiv:1908.05993 source file (2019-08-16)
Supplement: Supplementary file 1 [file appendix.tex]

\appendix
\section*{Appendix}

The effective area for this search, corresponding to the efficiency of the analysis cuts to reject the atmospheric muon background, together with the angular resolution, determines the sensitivity of this search.  The expected signal rate of muon neutrinos and anti-neutrinos ($\frac{dN_{\nu+\bar{\nu}}}{dt}$) from a point-like source at declination $\delta$ from a flux ($\phi_{\nu+\bar{\nu}}$) as a function of neutrino energy ($E_\nu$), averaged over the solid angle ($\Omega$) containing the declination $\delta$ is:
\begin{equation}
    \frac{dN_{\nu+\bar{\nu}}}{dt}=\int d\Omega\int_0^\infty A_{eff}^{\nu+\bar{\nu}}(E_\nu,\Omega, \delta)\times \phi_{\nu+\bar{\nu}}(E,\Omega)\text dE { .}
\end{equation}

 \begin{figure}[hbt!]
    \centering
    \includegraphics[width=0.5\textwidth]{images/Energy_PDF.png}
    %\includesvg[width=0.5\textwidth]{images/IC86II_effA.svg}
    \caption{The 2D distribution of events in one year of data for the final event selection is shown as an example of a background energy PDF. The 90\% energy range for the data (black), as well as simulated astrophysical signal Monte-Carlo (MC) for an $E^{-2}$ and an $E^{-3}$ spectrum are shown in magenta and orange respectively as a guide for the relevant energy range of IceCube.}
    \label{fig:enPDF}
\end{figure}
